# Supplementary material for: Promises and Pitfalls of Threshold-based Auto-labeling
Source: arXiv:2211.12620 source file (2024-02-22)
Supplement: Supplementary file 1 [file backup.tex]

\mycomment{

  \begin{figure*}[ht]
  \vspace{-8pt}
  \centering
  \mbox{
    \subfigure[Performance with varying training data size. The validation size used here is 4k, error threshold $\epsilon_a=1\%$\label{fig:unit-ball-train}]{\includegraphics[scale=0.23]{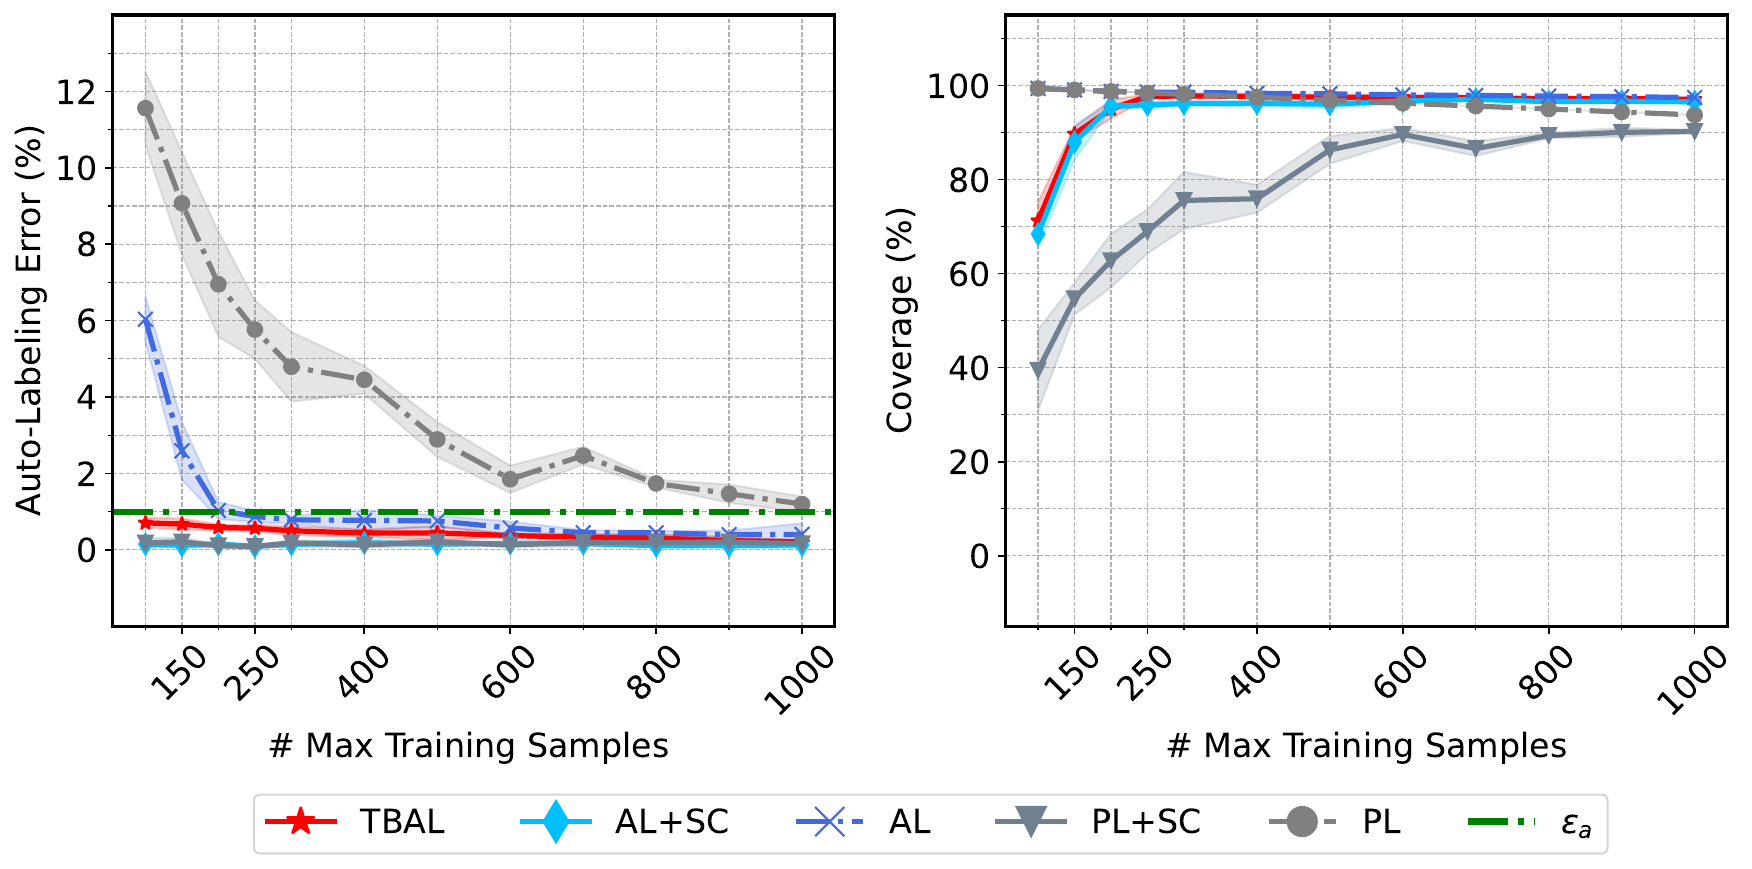}}\quad
    
    \subfigure[ Performance with varying validation data size. Max training samples = 500, error threshold $\epsilon_a=1\%$. \label{fig:unit-ball-val}]{\includegraphics[scale=0.23]{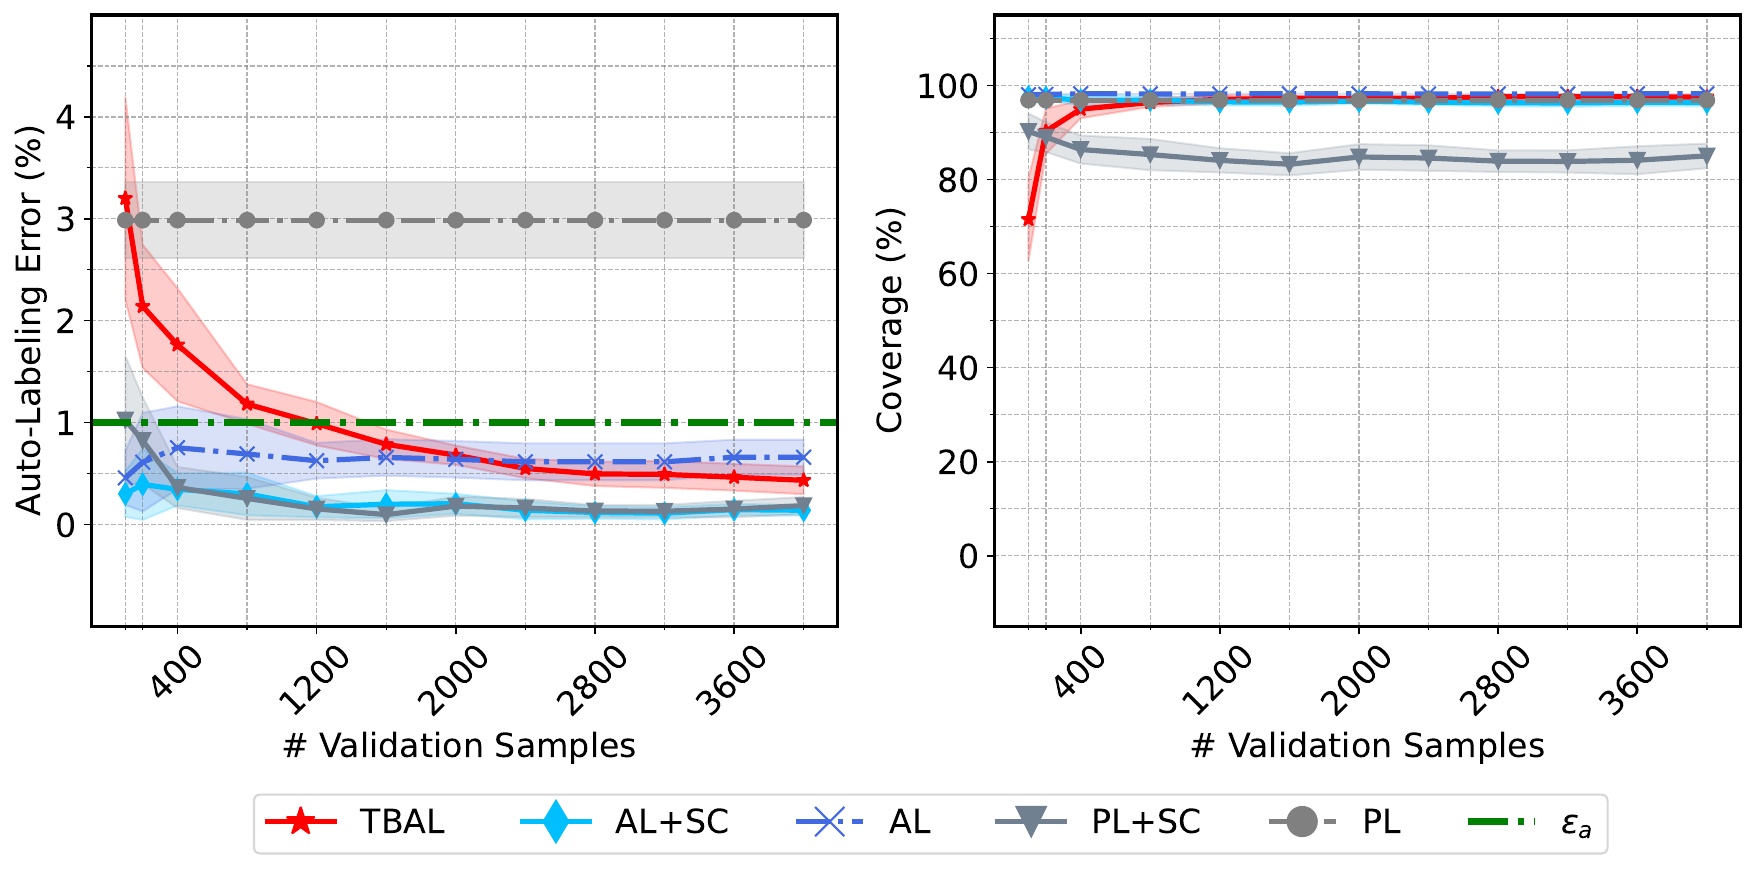}}
  }
\vspace{-8pt}
  \caption{ Auto-labeling performance on the Unit-Ball dataset. Left figure (a) We keep the validation data size the same for all methods and vary the training data size. In the right figure (b) we keep the training data size fixed and vary the validation data size. The lines show the mean and the shaded region shows 1-standard deviation estimated over 10 trials with different random seeds.  }
 
  \label{fig:unit-ball-exp}
\end{figure*}

}



  \begin{figure*}[t]
  \vspace{-8pt}
  \centering
  \mbox{
    \subfigure[ Varying validation data size with no UCB. Training size used here is 4k, $\epsilon_a=1\%$\label{fig:unit-ball-train}]{\includegraphics[scale=0.25]{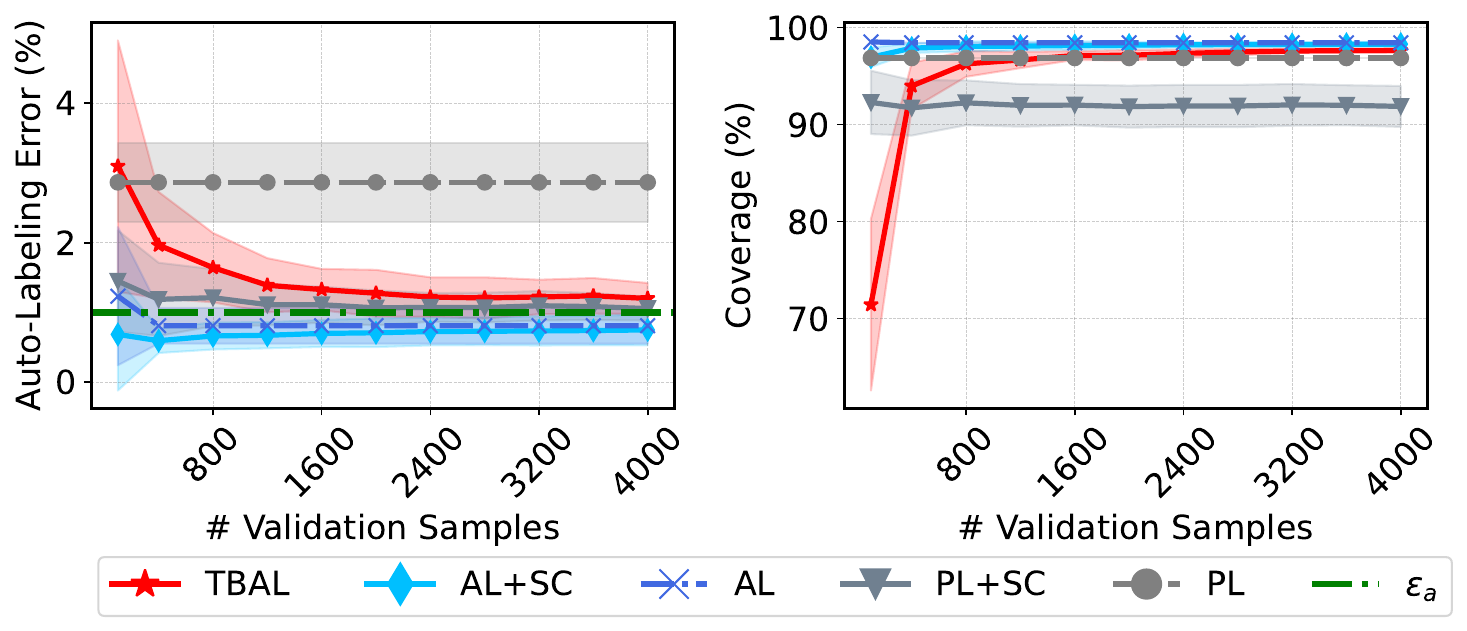}}\quad
    
    \subfigure[ Varying validation data size with UCB, $C_1 = 0.25$. Max training samples = 500, $\epsilon_a=1\%$. \label{fig:unit-ball-val}]{\includegraphics[scale=0.25]{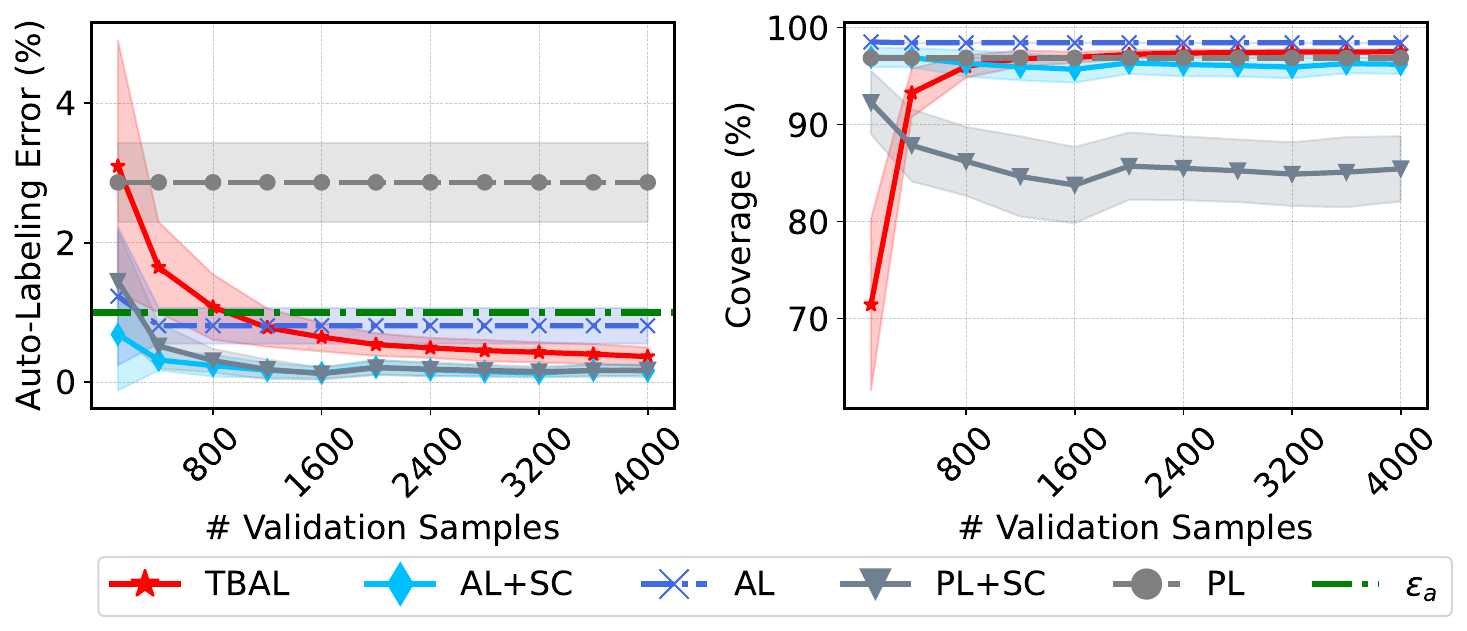}}
  }
\vspace{-8pt}
  \caption{ Auto-labeling performance on the Unit-Ball dataset. Left figure (a) We keep the validation data size the same for all methods and vary the training data size. In the right figure (b) we keep the training data size fixed and vary the validation data size. The lines show the mean and the shaded region shows 1-standard deviation estimated over 10 trials with different random seeds.  }
 
  \label{fig:unit-ball-exp}
\end{figure*}

%\vspace{-10pt}
\section{Experiments}\label{sec:experiments}
%\vspace{-5pt}
 We study the effectiveness of the TBAL algorithm on synthetic and real datasets. 
 %
 Our goal is to validate our theoretical results and understand the amount of labeled validation and training data required by the algorithm to achieve a certain auto-labeling error and coverage. 
 %
 We also seek to understand whether our findings apply to real data---where labels may be noisy---along with how well TBAL performs compared to common baselines.
 
 \begin{enumerate}
     \item 
 \end{enumerate}
 
 \textbf{Baselines:} We compare TBAL to the following methods: %that can be used to create auto-labeled datasets,\\
 %\begin{itemize}
     \textit{a. Passive Learning (PL)}: This method queries a subset of the points randomly to train a model from a given model class and then uses it to predict the labels for the remaining unlabeled pool.\\
     \textit{b. Active Learning (AL)}: This method uses active learning (using margin-random query strategy which is described below) to train a model from a given model class and then uses it to predict the labels for the remaining unlabeled pool.\\ 
      \textit{c. Passive Labeling + Selective Classification (PL+SC) } This method first performs passive learning to train a model from a given model class. Then it performs auto-labeling on the unlabeled using threshold-based selective classification with the model output by passive learning. So, only those unlabeled points that are deemed as fit to be labeled by the selection function are auto-labeled.\\
      \textit{d. Active Learning + Selective Classification (AL+SC): } This method first performs active learning (using margin-random query strategy which is described below) to train a model from a given model class.
     Then it performs auto-labeling using threshold-based selective classification with the model output by active learning.\\
 %\end{itemize}
 For  selective classification in the above methods, we use  Algorithm \ref{alg:gamma-estimate} to estimate the threshold and use it to perform auto-labeling. In experiments, we adapt Algorithm \ref{alg:gamma-estimate} slightly---instead of estimating a single threshold for all classes, we  estimate thresholds for each class separately.
 
\textbf{Active Querying Strategy :}\label{para:querystrategy}
We use the \emph{margin-random} query strategy for querying the next batch of training data. In this strategy, the algorithm first sorts the points based on the margin (uncertainty) score and then selects the top $C n_b$ ($C>1$) points from which $n_b$ points are picked at random. This is a simple and computationally efficient method that balances the exploration and exploitation trade-off. We note that other active-querying strategies exist; we use margin-random as our standard querying strategy to keep the focus on comparing auto-labeling---not active learning approaches. %We note that there are other active-querying strategies e.g. \cite{} which use clustering on features of the penultimate layer of the network. Since we are studying auto-labeling algorithms and our goal is not to compare different active-querying strategies we chose to use \emph{margin-random}.

%Getting good clustering depends on good features and one needs enough labeled data to first get good features.

\begin{figure*}[ht]
% CIFAR-10 Medium Net
\vspace{-4mm}
  \centering
  \mbox{
    \subfigure[ Varying training data size\label{fig:cifar10-mednet-train} while keeping validation size = 10k, $\epsilon_a$ = 10\%.]{\includegraphics[height=28mm,scale=0.23]{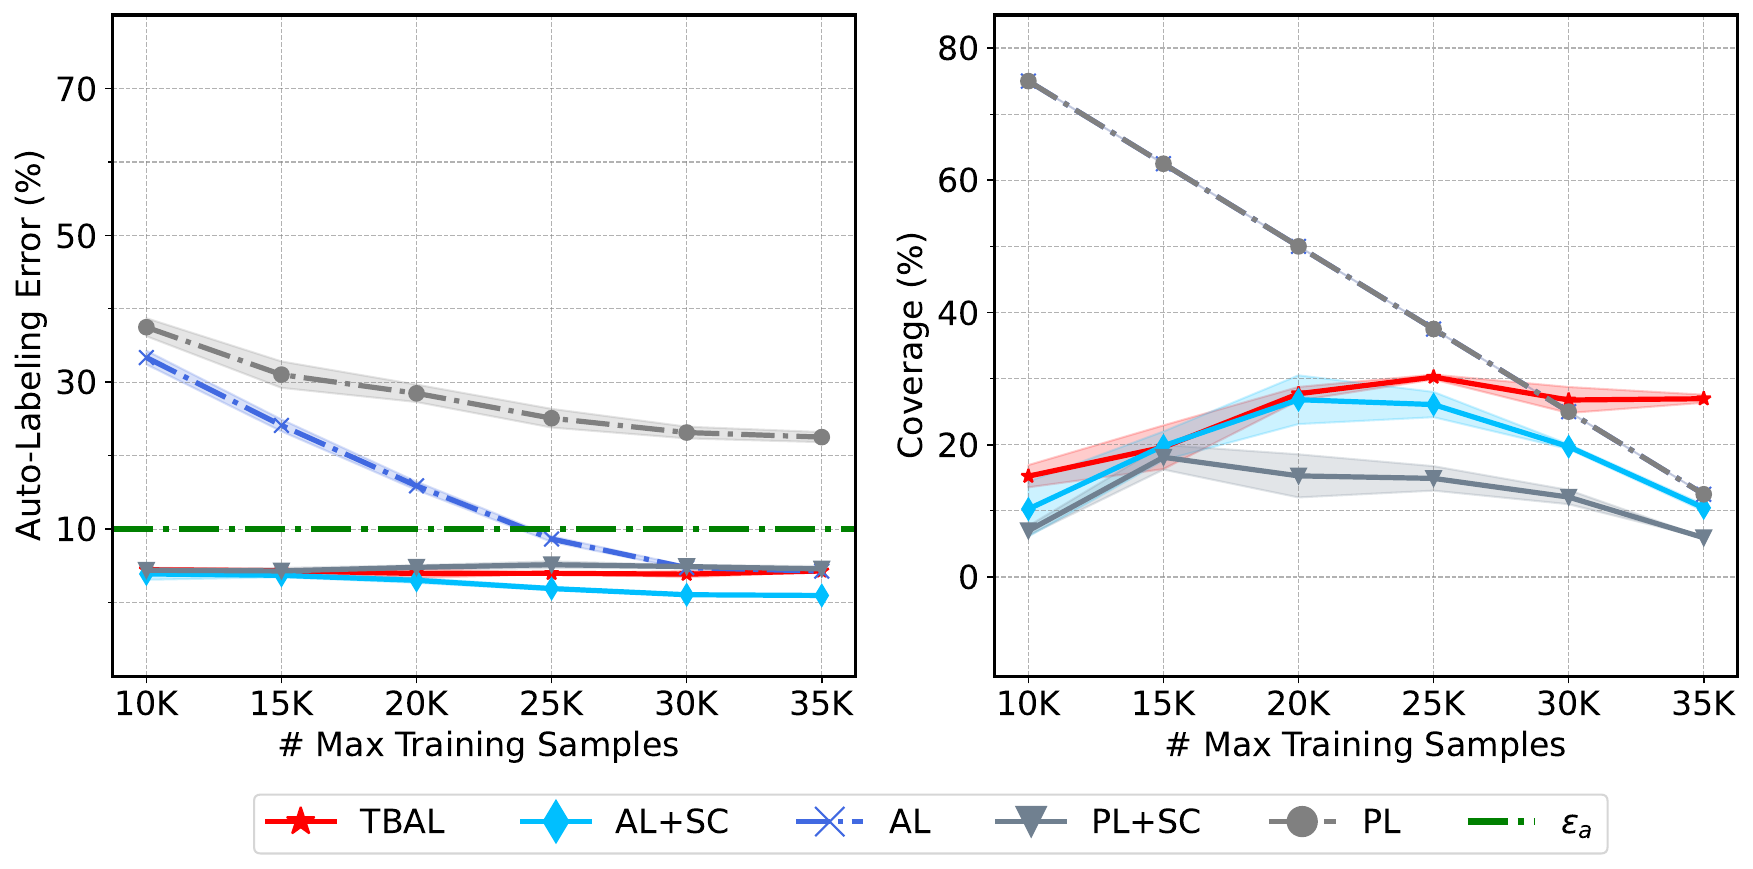}}\quad
    
    \subfigure[ Varying validation  size, while keeping training data size = 20k, $\epsilon_a$= 10\%. \label{fig:cifar10-mednet-val}]{\includegraphics[height=28mm,scale=0.23]{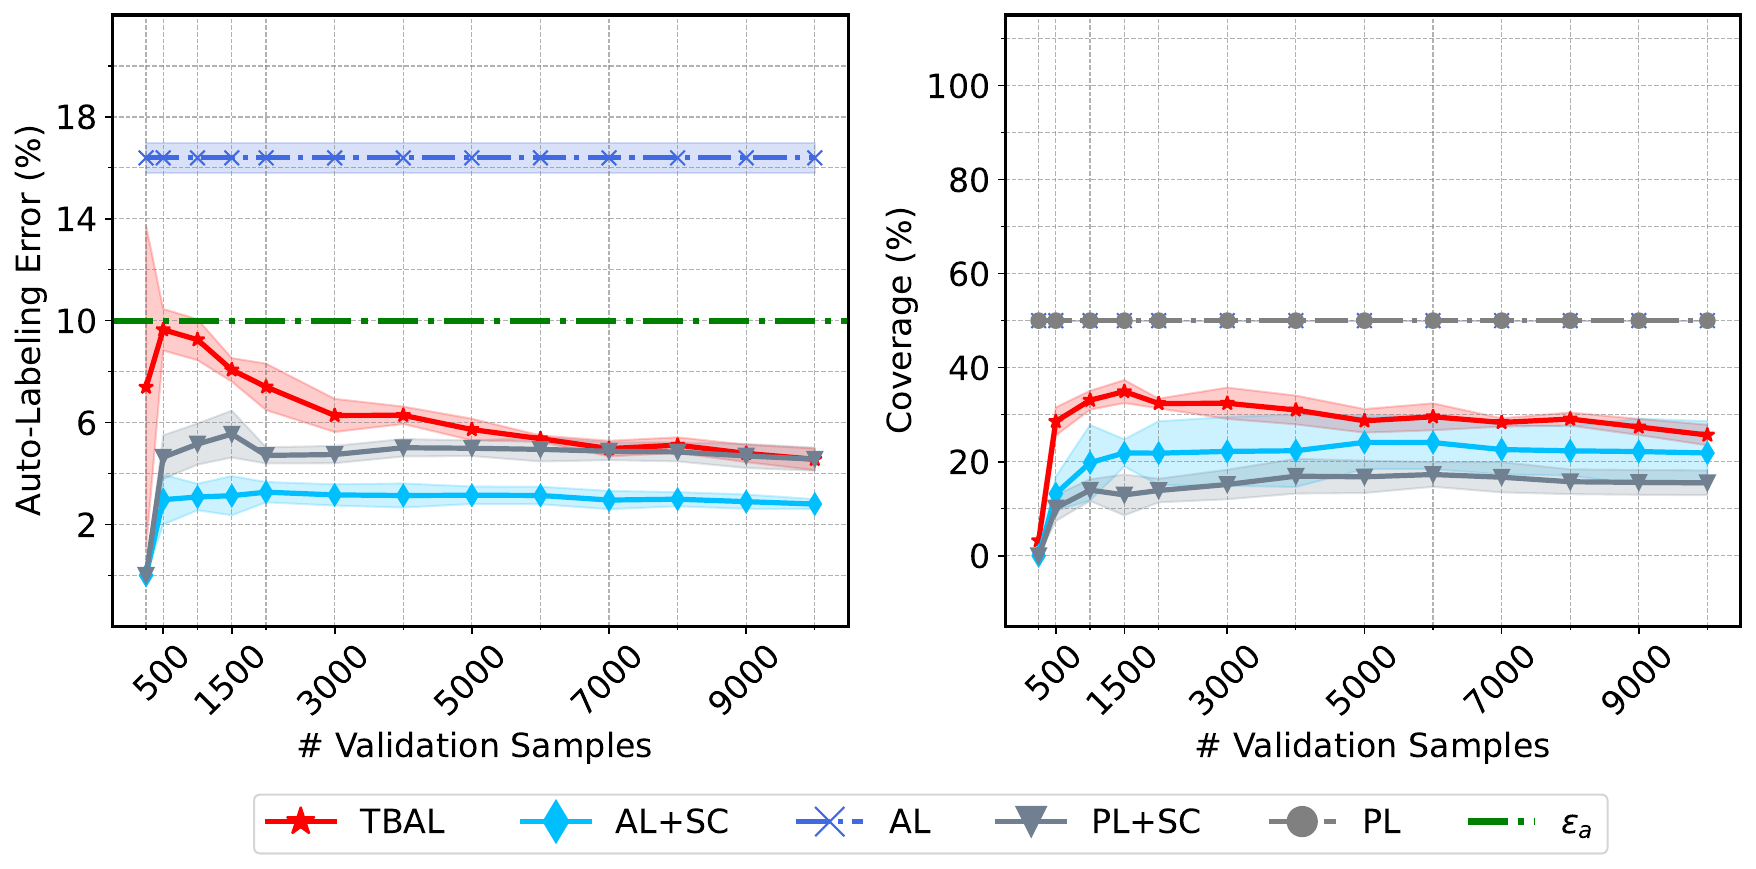}}
  }
  \vspace{-2mm}
  \caption{ Effect of training  and validation data size on auto-labeling performance on CIFAR-10 dataset using a medium-sized CNN network. $X_{pool} $ and $X_{val}$ are created by splitting the standard 50k train points into 40k and 10k points respectively. Figures show the mean and std. deviation observed over 5 trials with different random seeds.  }
  \label{fig:cifar10-mednet-exp}
  \vspace{-5pt}
\end{figure*}
 \textbf{Datasets:} We use five datasets, three synthetic and two real. For each dataset, we split the data into two sufficiently large pools. One is used as $X_{pool}$ on which auto-labeling algorithms are run and the other is used as $X_{val}$ from which the algorithms subsample validation data. Here we discuss the results on three of them and others are discussed in the appendix(Section \ref{sec:additional-exp}).
 The datasets are\\
 %\begin{itemize}
\textit{a. Unit-Ball} is a synthetic dataset of uniformly sampled points from the $d$-dimensional unit ball. The true labels are generated using a homogeneous linear separator with $\bw = [1/\sqrt{d},\ldots,1/\sqrt{d}]$. We use $d=30$ and generate N=20k samples, out of which 16k are in $X_{pool}$ and 4k are in $X_{val}$. 

\textit{b. Circles} is a synthetic dataset where $\cX$ consists of points 2D points on two concentric circles, each corresponding to a class. It is created using \texttt{make\_circles} function of \texttt{sklearn}. We generate N=10k samples, out of which we keep 16k in $X_{pool}$ and create a validation pool $X_{val}$ of size 4k.

\textit{c. CIFAR-10}~\cite{krizhevsky2009learning} is an image dataset of 10 classes. We randomly split the standard training set into $X_{pool}$ of size 40k and the validation pool of size 10k.

 %We conduct additional experiments on the MNIST and XOR datasets. 
 \textbf{Models and Training}:
 For the linear models, we use SVM with the usual hinge loss and train it till loss tolerance 1e-5. To train medium CNN net we use SGD with a learning rate of 1e-2, batch size 256, and momentum of 0.9. More details on the model training are in the supplementary material.

For SVMs we use the standard implementations of \cite{wu2003probability,platt1999SVM-Prob} in  \texttt{sklearn}   to get the prediction probabilities and use them as the score function. For neural networks, we use softmax output as the score function. We also consider an energy-based scoring function  \cite{lecun2006tutorial-energy} in Sec.~\ref{subsec:confidence-exp}.

 \mycomment{CIFAR-10 dataset (Figure \ref{fig:cifar10-mednet-exp}). We perform auto-labeling using a medium-sized CNN network with 6 convolution layers followed by 3 linear layers. We study the role of training data size (see Figure \ref{fig:cifar10-mednet-train}) and validation data size (see Figure \ref{fig:cifar10-mednet-val}). We observe that TBAL does better than AL+SC with more training data since AL could not converge to a classifier with an error < 10\% and used the full training budget. Due to differences in the dynamics, TBAL achieves better coverage. In Figure \ref{fig:cifar10-mednet-val} we see the effect of validation data size. As expected it impacts TBAL more, especially when the validation data is too little. \\
\textbf{(d) Clarity and Typos:} Thanks for the suggestions, we have incorporated the feedback and updated the draft accordingly.}
 %\subsection{ Results and Discussion:}
\vspace{-5pt}
\subsection{Role of Validation Data}
We study the role of validation data in the auto-labeling performance of the methods. % expectation..
%\rkv{Do these experiments run only on TBAL or also on baselines?}
% 
 As the validation data plays a crucial role in determining the threshold for automatically labeling points with confidence, we expect the accuracy of auto-labeled points will decrease with less validation data.

\textbf{Setup:}
We study this on the Unit-Ball and CIFAR-10 datasets. We keep the maximum training data size $N_q$=500 and 20k and the auto-labeling error threshold  $\epsilon_a$ = 1\% and 10\% respectively for the    Unit-Ball and 20k for CIFAR-10 datasets.  We vary the validation data size given to the algorithms.  Initial seed data of size $n_s$ is 20\% of $N_q$ and query batch size $n_b$ is $5\%$ of $N_q$ and $C=2$ for both AL and TBAL for both datasets. We give the same initial seed samples of size $n_s$ to all the methods to ensure they get the same starting point. 


\begin{figure*}[ht]
% CIFAR-10 Medium Net
\vspace{-4mm}
  \centering
  \mbox{
    \subfigure[ (IMDB) Varying training data size\label{fig:cifar10-mednet-train} while keeping validation size = 10k, $\epsilon_a$ = 5\%.]{\includegraphics[height=28mm,scale=0.23]{figures/v3/imdb_val_eps_0.05_c1_0_nq_2000.pdf}}\quad
    %figures/v3/imdb_n_q_eps_0.05_c1_0.25_nv_5000.pdf
    \subfigure[ (IMDB)Varying validation  size, while keeping training data size = 20k, $\epsilon_a$= 5\%. \label{fig:cifar10-mednet-val}]{\includegraphics[height=28mm,scale=0.23]{figures/v3/imdb_val_eps_0.05_c1_0.25_nq_2000.pdf}}
  }
  \vspace{-2mm}
  \caption{IMDB}
  \label{fig:cifar10-mednet-exp}
  \vspace{-5pt}
\end{figure*}


\begin{figure*}[ht]
% CIFAR-10 Medium Net
\vspace{-4mm}
  \centering
  \mbox{
    \subfigure[ (Imagenet) Varying validation  size size\label{fig:cifar10-mednet-train} while keeping training size = 10k, $\epsilon_a$ = 10\%.]{\includegraphics[height=28mm,scale=0.23]{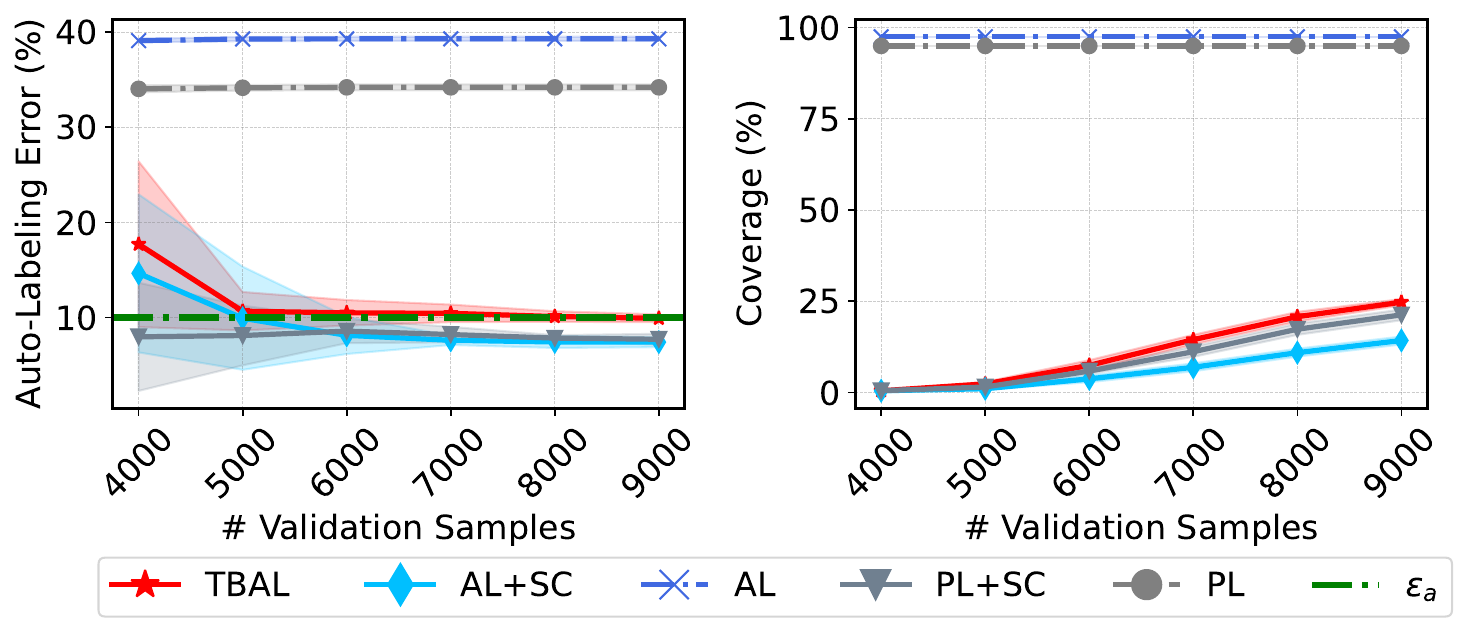
    }}\quad
    %figures/v3/imdb_n_q_eps_0.05_c1_0.25_nv_5000.pdf
    \subfigure[ (Imagenet) Varying validation  size, while keeping training data size = 20k, $\epsilon_a$= 10\%. \label{fig:cifar10-mednet-val}]{\includegraphics[height=28mm,scale=0.23]{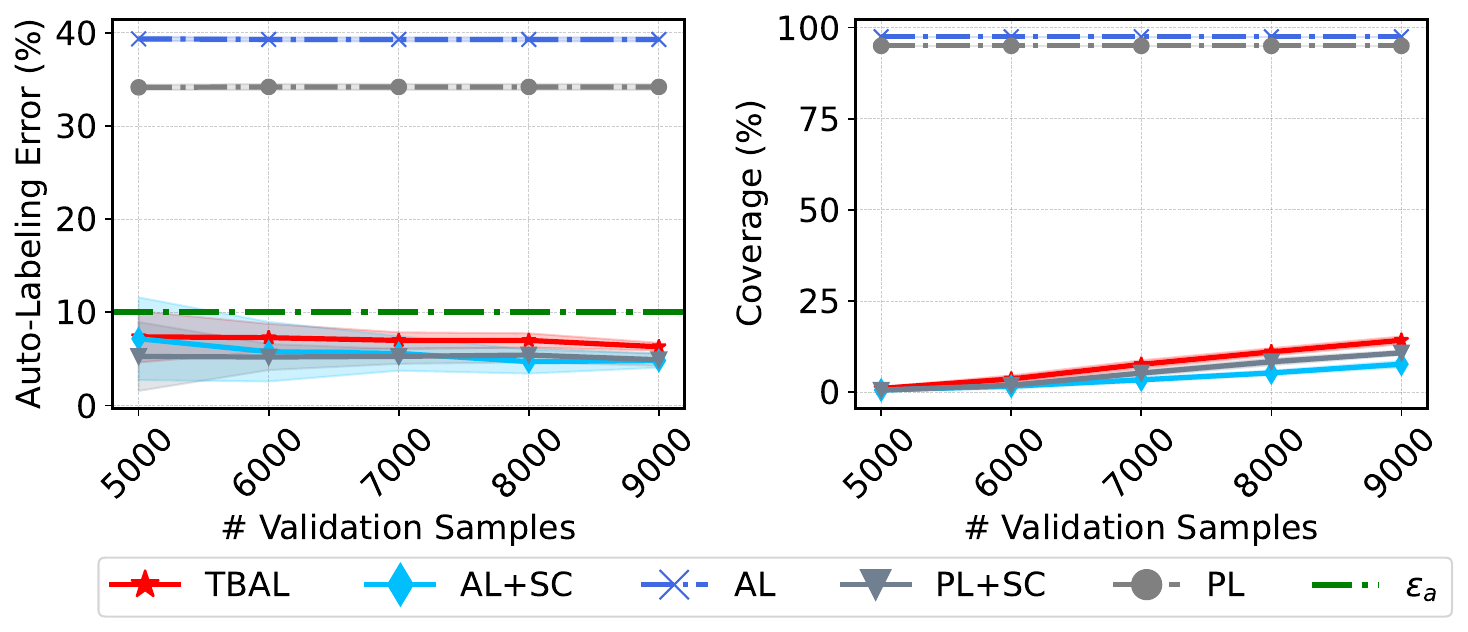}}
  }
  \vspace{-2mm}
  \caption{Tiny Imagenet}
  \label{fig:cifar10-mednet-exp}
  \vspace{-5pt}
\end{figure*}

%\textbf{Results:} Figure \ref{fig:unit-ball-val} and \ref{fig:cifar10-mednet-val} show the auto-labeling error and the coverage achieved by TBAL and other algorithms on the Unit-Ball and CIFAR-10 datasets respectively. As expected, if the validation data provided to the TBAL algorithm is insufficient, the resulting auto-labeling error is higher. We observe that the auto-labeling error as well as the coverage of the TBAL algorithm improves as more validation data is used. Having too little $X_{val}$ leads to incorrect estimates of the auto-labeling error which makes the algorithm estimate incorrect thresholds leading to poor auto-labeling performance. This is also highlighted by our theoretical analysis (see Theorem~\ref{thm:general_auto_err_full}).
\textbf{Results:} The figures \ref{fig:unit-ball-val} and \ref{fig:cifar10-mednet-val} demonstrate the impact of validation data on the performance of the TBAL and other algorithms. As seen in the figures, the auto-labeling error and coverage of TBAL and other algorithms are affected by the amount of validation data provided. When the validation data is insufficient, the auto-labeling error of the TBAL algorithm increases. However, as more validation data is used, the auto-labeling error and coverage of the TBAL algorithm improve. Additionally, it is worth noting that providing too little $X_{val}$ can lead to incorrect estimates of the auto-labeling error, which in turn results in poor auto-labeling performance. This is further highlighted in our theoretical analysis as seen in Theorem~\ref{thm:general_auto_err_full}.
\vspace{-8pt}

\subsection{Role of Hypothesis Class}
%An important consideration is the choice of the function class used to perform auto-labeling. 
%In practice, one does not know the true function class. Choosing a powerful function class such as deep neural networks requires large amounts of labeled training samples which defeats the purpose of creating an auto-labeled dataset for future training purposes. Here we examine whether in less powerful hypothesis classes---in particular, where the best classifier in the class has a constant risk---it is possible to auto-label the data with high accuracy and reasonably large coverage.
An important factor to consider when in auto-labeling is the choice of function class used. In real-world scenarios, the true function class is often unknown. Using powerful function classes like deep neural networks can be beneficial but can also require a large amount of labeled training data, which can be counter-productive when the goal is to create an auto-labeled dataset for future use. In this context, we investigate whether using less powerful hypothesis classes can still achieve high accuracy and reasonable coverage in the auto-labeling process. 
%In particular, we focus on cases where the best classifier in the class has a constant risk.
%We study the question is it possible to auto-label the data with high accuracy and coverage using a less powerful hypothesis class (e.g. linear classifiers) 

\textbf{Setup:} We study this question by performing auto-labeling using  linear classifiers in the settings where the data is not linearly separable -- on Circles,  MNIST, and another synthetic dataset. Here we present the results for Circles dataset setting (described in Section~\ref{sec:autolabelingComparisons}), others are discussed in the appendix(\ref{sec:additional-exp}). For the Circles dataset, we use $n_s=16, n_b=8$ and $C=2$.

\textbf{Results:} 
Figure \ref{fig:circles-main} shows the auto-labeling performance on the Circles dataset using linear classifiers as the hypothesis class. We can see that TBAL is able to achieve high accuracy in auto-labeling the data on this dataset while other methods (notably AL+SC) are performing poorly. 
\vspace{-5pt}
\subsection{Role of Training Data Size}
%The algorithms query labels for the part of the unlabeled pool to train model and use it for auto-labeling and thus it becomes an important part of the overall data labeling cost. 

%\begin{figure}[!h]
%\includegraphics[width=0.45\textwidth]{figures/CIFAR10/cifar10_resnet18_18_fig_comparison_plot.pdf}
%\caption{Auto-labeling performance on the CIFAR-10 dataset. We keep validation data size same and vary the training data size. The auto-labeling error threshold $\epsilon_a=0.3$.}
%\end{figure} 

The labels queried for model training also play an important role and incur costs in the process. The next experiment focuses on the impact of training data on auto-labeling.

\textbf{Setup:} We limit the amount of training data the algorithm can use and observe the auto-labeling error and coverage. We ensure all the algorithms have sufficiently large but equal amounts of validation data. We run this experiment on all five datasets. We use the same values of $n_s$ and $n_b$ and $C$ as in previous experiments.

\textbf{Results:}  Our results, presented in figures ~\ref{fig:unit-ball-train}, ~\ref{fig:circles-plot}, ~\ref{fig:cifar10-mednet-train} ~\ref{fig:xor-plot}, and\ref{fig:mnist-exp}, indicate that TBAL and methods utilizing selective classification (AL+SC, PL+SC) maintain a high level of accuracy, even in scenarios where minimal training samples are used. It is expected since the threshold estimation method (when used with sufficient validation data) will find auto-labeling thresholds such that the auto-labeling error does not exceed $\epsilon_a$. The impact of training data size can be seen clearly in the coverage achieved by the algorithms. As expected, with fewer training samples the model has low accuracy leading to low coverage. However, as more samples are acquired, a more accurate model within the function class is learned, resulting in increased coverage.

%Active learning literature is full of querying strategies that minimize the 
%\comment{

%\begin{figure*}[h]
%  \centering
%  \mbox{
%    \subfigure[Auto-Labeling Error \label{subfigure label}]{\includegraphics[scale=0.4]{figures/unit-ball-exp/unitball-error-rate.pdf}}\quad
%    \subfigure[Auto-Labeling Coverage \label{subfigure label}]{\includegraphics[scale=0.4]{figures/unit-ball-exp/unitball-coverage.pdf}}\quad
   % \subfigure[Labeling Performance of various methods (TO BE UPDATED)\label{subfigure label}]{\includegraphics[scale=0.25]{figures/xor-exp/xor-comparison.pdf}}
 % }
 % \caption{Placeholder figure.}
 % \label{main figure label}
%\end{figure*}

%\subsection{Understanding Training Data Requirements}


%mnist_linear_fig_comparison_plot.pdf



 \mbox{
    \subfigure[ (CIFAR-10) Varying training data (Change fig new dims) size\label{fig:cifar10-mednet-train} while keeping validation size = 10k, $\epsilon_a$ = 10\%.]{\includegraphics[scale=0.275]{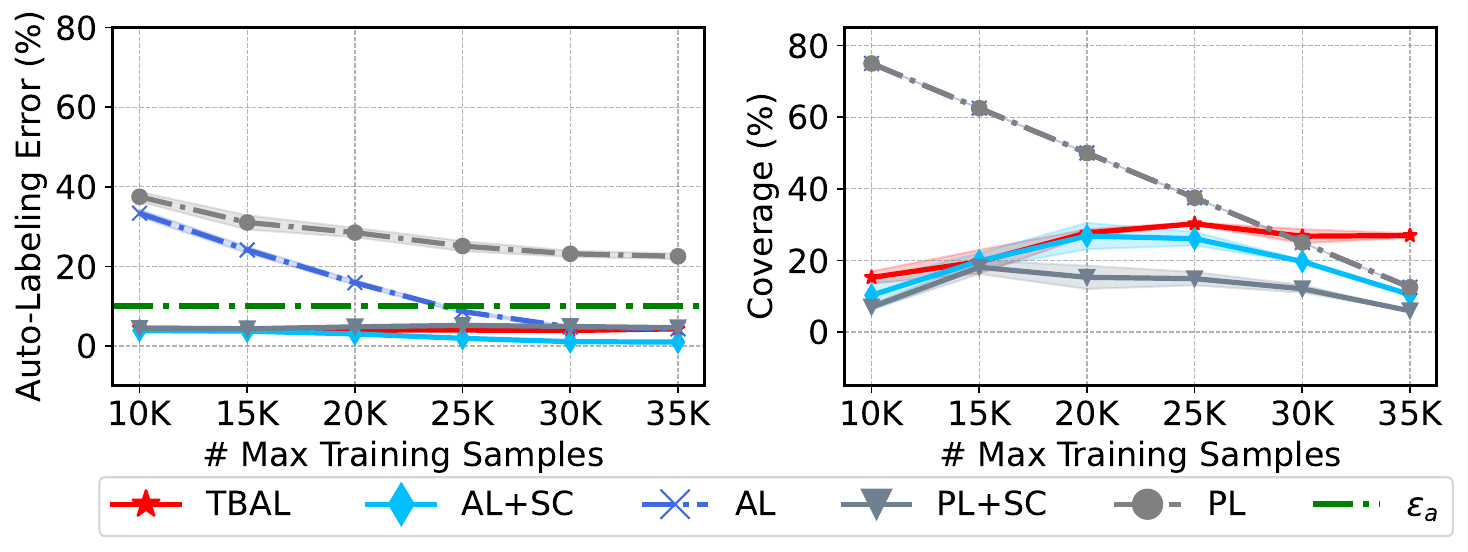}}\quad
    %figures/v3/imdb_n_q_eps_0.05_c1_0.25_nv_5000.pdf
    \subfigure[ (Tiny-Imagenet) Training data  $\epsilon_a$= 10\%. \label{fig:imgnet-train}]{\includegraphics[scale=0.275]{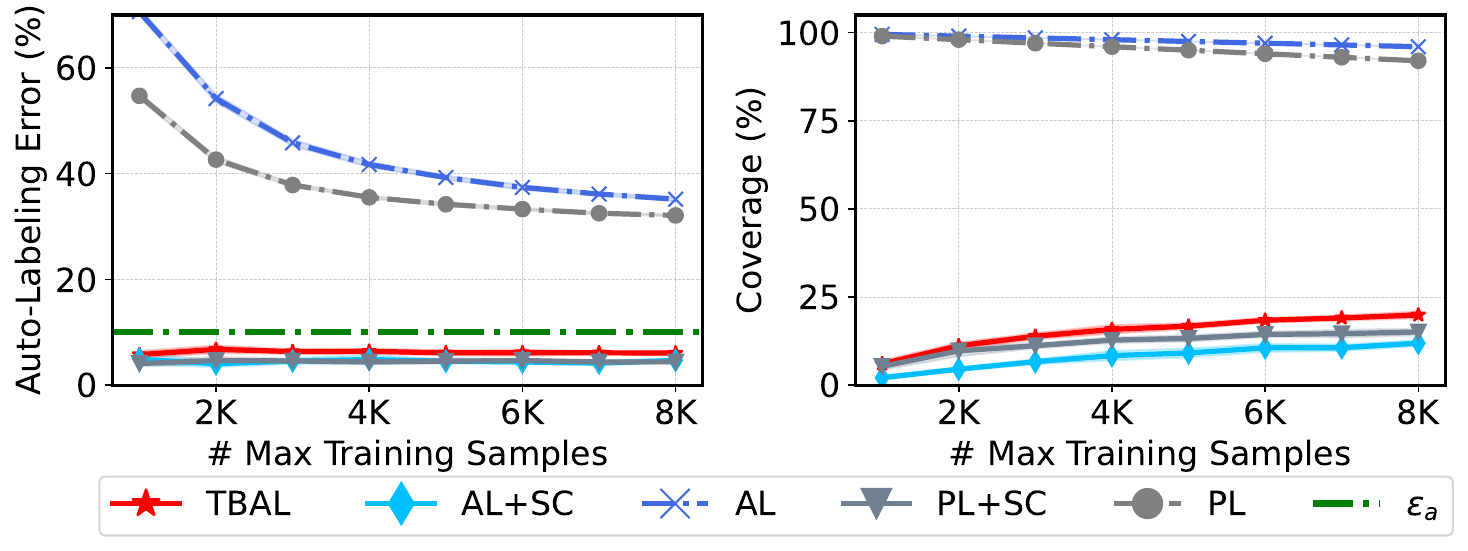}}
    
  }
